# Supplementary material for: A Diamond Quantum Oscilloscope
Source: arXiv:2105.06037 source file (2026-11-17)
Supplement: Supplementary file 1 [file sm.tex]

\documentclass[onecolumn,superscriptaddress,longbibliography,12pt]{revtex4}
%%%%%%%%%%%%%%%%%%%%%%%%%%%%%%%%%%%%%%%%%%%%%%%%%%%%%%%%%%%%%%%%%%%%%%%%%%%%%%%%%%%%%%%%%%%%%%%%%%%%%%%%%%%%%%%%%%%%%%%%%%%%%%%%%%%%%%%%%%%%%%%%%%%%%%%%%%%%%%%%%%%%%%%%%%%%%%%%%%%%%%%%%%%%%%%%%%%%%%%%%%%%%%%%%%%%%%%%%%%%%%%%%%%%%%%%%%%%%%%%%%%%%%%%%%%%
\usepackage{graphicx}
\usepackage{amssymb}
\usepackage{amsmath}
\usepackage{epsfig}
\usepackage{color}
\usepackage{natbib}
\usepackage{mathtools}
\usepackage[colorlinks,linkcolor=blue,anchorcolor=blue,citecolor=blue,urlcolor=blue]{hyperref}
\usepackage[left]{lineno}
\usepackage{blindtext}
\usepackage{color, soul}
\usepackage{setspace}
\usepackage{fancyhdr}
\usepackage{enumerate}
\begin{document}

\setulcolor{red}

\title{Supplemental Material: Heisenberg-Limited Waveform Estimation with Solid-State Spins in Diamond}
\author{Yang Dong}
\author{Ze-Hao Wang}
\author{Hao-Bin Lin}
\author{Shao-Chun Zhang}
\author{Yu Zheng}
\affiliation{{CAS Key Laboratory of Quantum Information, University of Science and Technology of China, Hefei, 230026, P.R. China}}
\affiliation{{CAS Center for Excellence in Quantum Information and Quantum Physics, University of Science and Technology of China, Hefei, 230026, P.R. China}}
\author{Xiang-Dong Chen}
\author{Wei Zhu}
\author{Guan-Zhong Wang}
\affiliation{{Hefei National Laboratory for Physical Science at Microscale, and Department of Physics, University of Science and Technology of China, Hefei, Anhui 230026, P. R. China}}
\author{Guang-Can Guo}
\author{Fang-Wen Sun}
\email{fwsun@ustc.edu.cn}
\affiliation{{CAS Key Laboratory of Quantum Information, University of Science and Technology of China, Hefei, 230026, P.R. China}}
\affiliation{{CAS Center for Excellence in Quantum Information and Quantum Physics, University of Science and Technology of China, Hefei, 230026, P.R. China}}
\maketitle

\makeatletter
\renewcommand{\thefigure}{S\@arabic\c@figure}
\makeatother
%\makeatletter
%\renewcommand{\thetable}{S\@arabic\c@table}
%\makeatother
\makeatletter
\renewcommand{\theequation}{S\@arabic\c@equation}
\makeatother
\section{The estimation error of waveform based on the least square method}

With the standard measurement scheme, we estimate the unknown waveform based
on $N = {n_1}{n_2}$ measurement results. In the present case, the overall results can be divided
into $n_1$ equal parts according to sampling time. For the sampling instant $t_i$, we have a serial
outputs ${\left\{ {{\phi _{i,j}}} \right\}}$ to get the unknown phase, where $i = 1,2, \cdots {n_1}$ and $j = 1,2, \cdots {n_2}$. Hence, the total estimation error of waveform
have a simple form:
\begin{equation}
\begin{aligned}
{\delta ^2} =& {\Bbb E}\left[ {\int_0^T {\frac{{dt}}{T}{{\left[ {\widetilde \phi  \left( t \right) - \phi \left( t \right)} \right]}^2}} } \right]\\
            =& \frac{1}{{{n_2}}}\sum\nolimits_{j = 1}^{{n_2}} {\left[ {\int_0^T {\frac{{dt}}{T}{{\left( {\sum\nolimits_{i = 1}^{{n_1}} {{\phi _{i,j}}\theta (t - {t_i})}  - \phi \left( t \right)} \right)}^2}} } \right]}   \\
            =& \frac{1}{{{n_2}}}\sum\nolimits_{j = 1}^{{n_2}} {\sum\nolimits_{i = 1}^{{n_1}} {\int_{{t_i} - \frac{T}{{2{n_1}}}}^{{t_i} + \frac{T}{{2{n_1}}}} {\frac{{dt}}{T}} } {{\left[ {{\phi _{i,j}} - \phi \left( t \right)} \right]}^2}}  \\
            =& \sum\nolimits_{i = 1}^{{n_1}} {\left[ {\frac{1}{{{n_2}}}\sum\nolimits_{j = 1}^{{n_2}} {\int_{{t_i} - \frac{T}{{2{n_1}}}}^{{t_i} + \frac{T}{{2{n_1}}}} {\frac{{dt}}{T}} } {{\left[ {{\phi _{i,j}} - {{\bar \phi }_i} + {{\bar \phi }_i} - \phi \left( t \right)} \right]}^2}} \right]} \text{,}
\end{aligned}
\end{equation}
where we define ${{\bar \phi }_i} = \frac{1}{{{n_2}}}\sum\nolimits_{j = 1}^{{n_2}} {{\phi _{i,j}}} $ based on the least square method. In this way, the
cross-term is zero:
\[\sum\nolimits_{i = 1}^{{n_1}} {\left[ {\frac{1}{{{n_2}}}\sum\nolimits_{j = 1}^{{n_2}} {\int_{{t_i} - \frac{T}{{2{n_1}}}}^{{t_i} + \frac{T}{{2{n_1}}}} {\frac{{dt}}{T}} } 2\left( {{\phi _{i,j}} - {{\bar \phi }_i}} \right)\left( {{{\bar \phi }_i} - \phi \left( t \right)} \right)} \right]} {\rm{ = }}0.\]
And we have
\begin{equation}
\begin{aligned}
{\delta ^2} =& \sum\nolimits_{i = 1}^{{n_1}} {\left[ {\frac{1}{{{n_2}}}\sum\nolimits_{j = 1}^{{n_2}} {\int_{{t_i} - \frac{T}{{2{n_1}}}}^{{t_i} + \frac{T}{{2{n_1}}}} {\frac{{dt}}{T}} } {{\left( {{\phi _{i,j}} - {{\bar \phi }_i}} \right)}^2} + \frac{1}{{{n_2}}}\sum\nolimits_{j = 1}^{{n_2}} {\int_{{t_i} - \frac{T}{{2{n_1}}}}^{{t_i} + \frac{T}{{2{n_1}}}} {\frac{{dt}}{T}} } {{\left( {{{\bar \phi }_i} - \phi \left( t \right)} \right)}^2}} \right]} \\
=& \sum\nolimits_{i = 1}^{{n_1}} {\left[ {\int_{{t_i} - \frac{T}{{2{n_1}}}}^{{t_i} + \frac{T}{{2{n_1}}}} {\frac{{dt}}{T}} \delta _{i,stat}^2 + \int_{{t_i} - \frac{T}{{2{n_1}}}}^{{t_i} + \frac{T}{{2{n_1}}}} {\frac{{dt}}{T}} \delta _{i,det}^2} \right]} \\
=& \frac{1}{{{n_1}}}\sum\nolimits_{i = 1}^{{n_1}} {\delta _{i,stat}^2}  + \sum\nolimits_{i = 1}^{{n_1}} {\int_{{t_i} - \frac{T}{{2{n_1}}}}^{{t_i} + \frac{T}{{2{n_1}}}} {\frac{{dt}}{T}} \delta _{i,det}^2}\\
=& \frac{1}{{{n_1}}}\sum\nolimits_{i = 1}^{{n_1}} {\delta _{i,stat}^2 + \int_0^T {\frac{{dt}}{T}} \delta _{i,det}^2} \\
=& \delta _{stat}^2{\rm{ + }}\delta _{det}^2 \text{,}
\end{aligned}
\end{equation}
where $\delta _{i,stat}^2{\text{ = }}\frac{1}{{{n_2}}}\sum\nolimits_{j = 1}^{{n_2}} {{{\left( {{\phi _{i,j}} - {{\bar \phi }_i}} \right)}^2}} $ and $\delta _{i,det}^2{\text{ = }}{\left( {{{\bar \phi }_i}\theta (t - {t_i}) - \phi \left( t \right)} \right)^2}$.

So the overall arbitrary waveform estimation error can be decomposed into two parts: the statistical
error $\delta _{stat}^2{\text{ = }}\frac{1}{{{n_1}}}\sum\nolimits_{i = 1}^{{n_2}} {\delta _{i,stat}^2} $ caused by the projection measurement and
the deterministic error $\delta _{det}^2{\text{ = }}\int_0^T {\frac{{dt}}{T}} \delta _{i,det}^2$ due to the smoothing process as shown in the main text. As
${n_2}$ increases large enough, the average measurement result ${\bar \phi _i}$ would converge to the ideal
value due to the central limit theorem. And for a finite number of experiment repeats, there will be some of the discrepancy between theory and experiment.
Under the restrictions of $\mathop {\sup }\limits_{0 < \varepsilon  < a} \int_0^T {\frac{{dt}}{T}{{\left| {\frac{{\phi \left( {t + \varepsilon } \right) - \phi \left( t \right)}}{{{\varepsilon ^q}}}} \right|}^2}} \leqslant \frac{{{M^2}}}{{{T^{2q}}}}$ for some positive number $M > 0$ \cite{PhysRevLett.124.010507}, we have the H\"{o}lder continuity ${\left| {\phi \left( {t + \varepsilon } \right) - \phi \left( t \right)} \right| = O\left( {{\varepsilon ^q}} \right)}$ equivalently. So once the average measurement results ${\bar \phi _i}$ converges to the ideal values of arbitrary waveform, the deterministic error scales as
\begin{equation}
\begin{aligned}
\delta _{det }^2 =& \sum\nolimits_{i = 1}^{{n_1}} {\int_{{t_i} - \frac{T}{{2{n_1}}}}^{{t_i} + \frac{T}{{2{n_1}}}} {\frac{{dt}}{T}} {{\left( {{{\bar \phi }_i}\theta (t - {t_i}) - \phi \left( t \right)} \right)}^2}} \\
=& \sum\nolimits_{i = 1}^{{n_1}} {\int_{ - \frac{T}{{2{n_1}}}}^{\frac{T}{{2{n_1}}}} {\frac{{dt}}{T}} O\left( {{t^{2q}}} \right)} \\
=& O\left( {n_1^{ - 2q}} \right) \text{.}
\end{aligned}
\end{equation}

For a given number of resources $N = {n_1}{n_2}$, the optimal measurement is determined by the trade-off between these errors. By employing the inequality of arithmetic and geometric means, the estimation error of arbitrary waveform is
\begin{equation}
\begin{aligned}
{\delta ^2}=& \delta _{det}^2 + \delta _{stat}^2\\
 =& O\left( {Mn_1^{ - 2q}} \right) + O\left( {n_2^{ - 1}} \right)\\
 \geqslant& O\left( {{{\left( {{M^{1/q}}{N^{ - 1}}} \right)}^{2q/(2q + 1)}}} \right)
\end{aligned}
\end{equation}
in SQL scheme. If we neglect the constant factor, we will get the optimal scaling relationship $\delta  = O\left( {{N^{ - q/(2q + 1)}}} \right)$ in the SQL scheme. With similar procedure, the total estimation error would be reduced with correlative quantum resources and scale as $\delta  = O\left( {{N^{ - q/(q + 1)}}} \right)$ in the HQL scheme. The optimal quantum resource allocation of arbitrary waveform estimation would meet this condition $n_1^{ - 2q} \sim n_2^{ - 1}$ for SQL and $n_1^{ - 2q} \sim n_2^{ - 2}$ for HQL with large $N$. And this relationship has a simple form: ${\log _2}{n_1} = \frac{1}{{2q}}{\log _2}{n_2} + {c_1}$ and ${\log _2}{n_1} = \frac{1}{q}{\log _2}{n_2} + {c_2}$ for SQL and HQL, respectively.

\begin{figure}[tbp]
\centering
\textsf{\includegraphics[width=11cm]{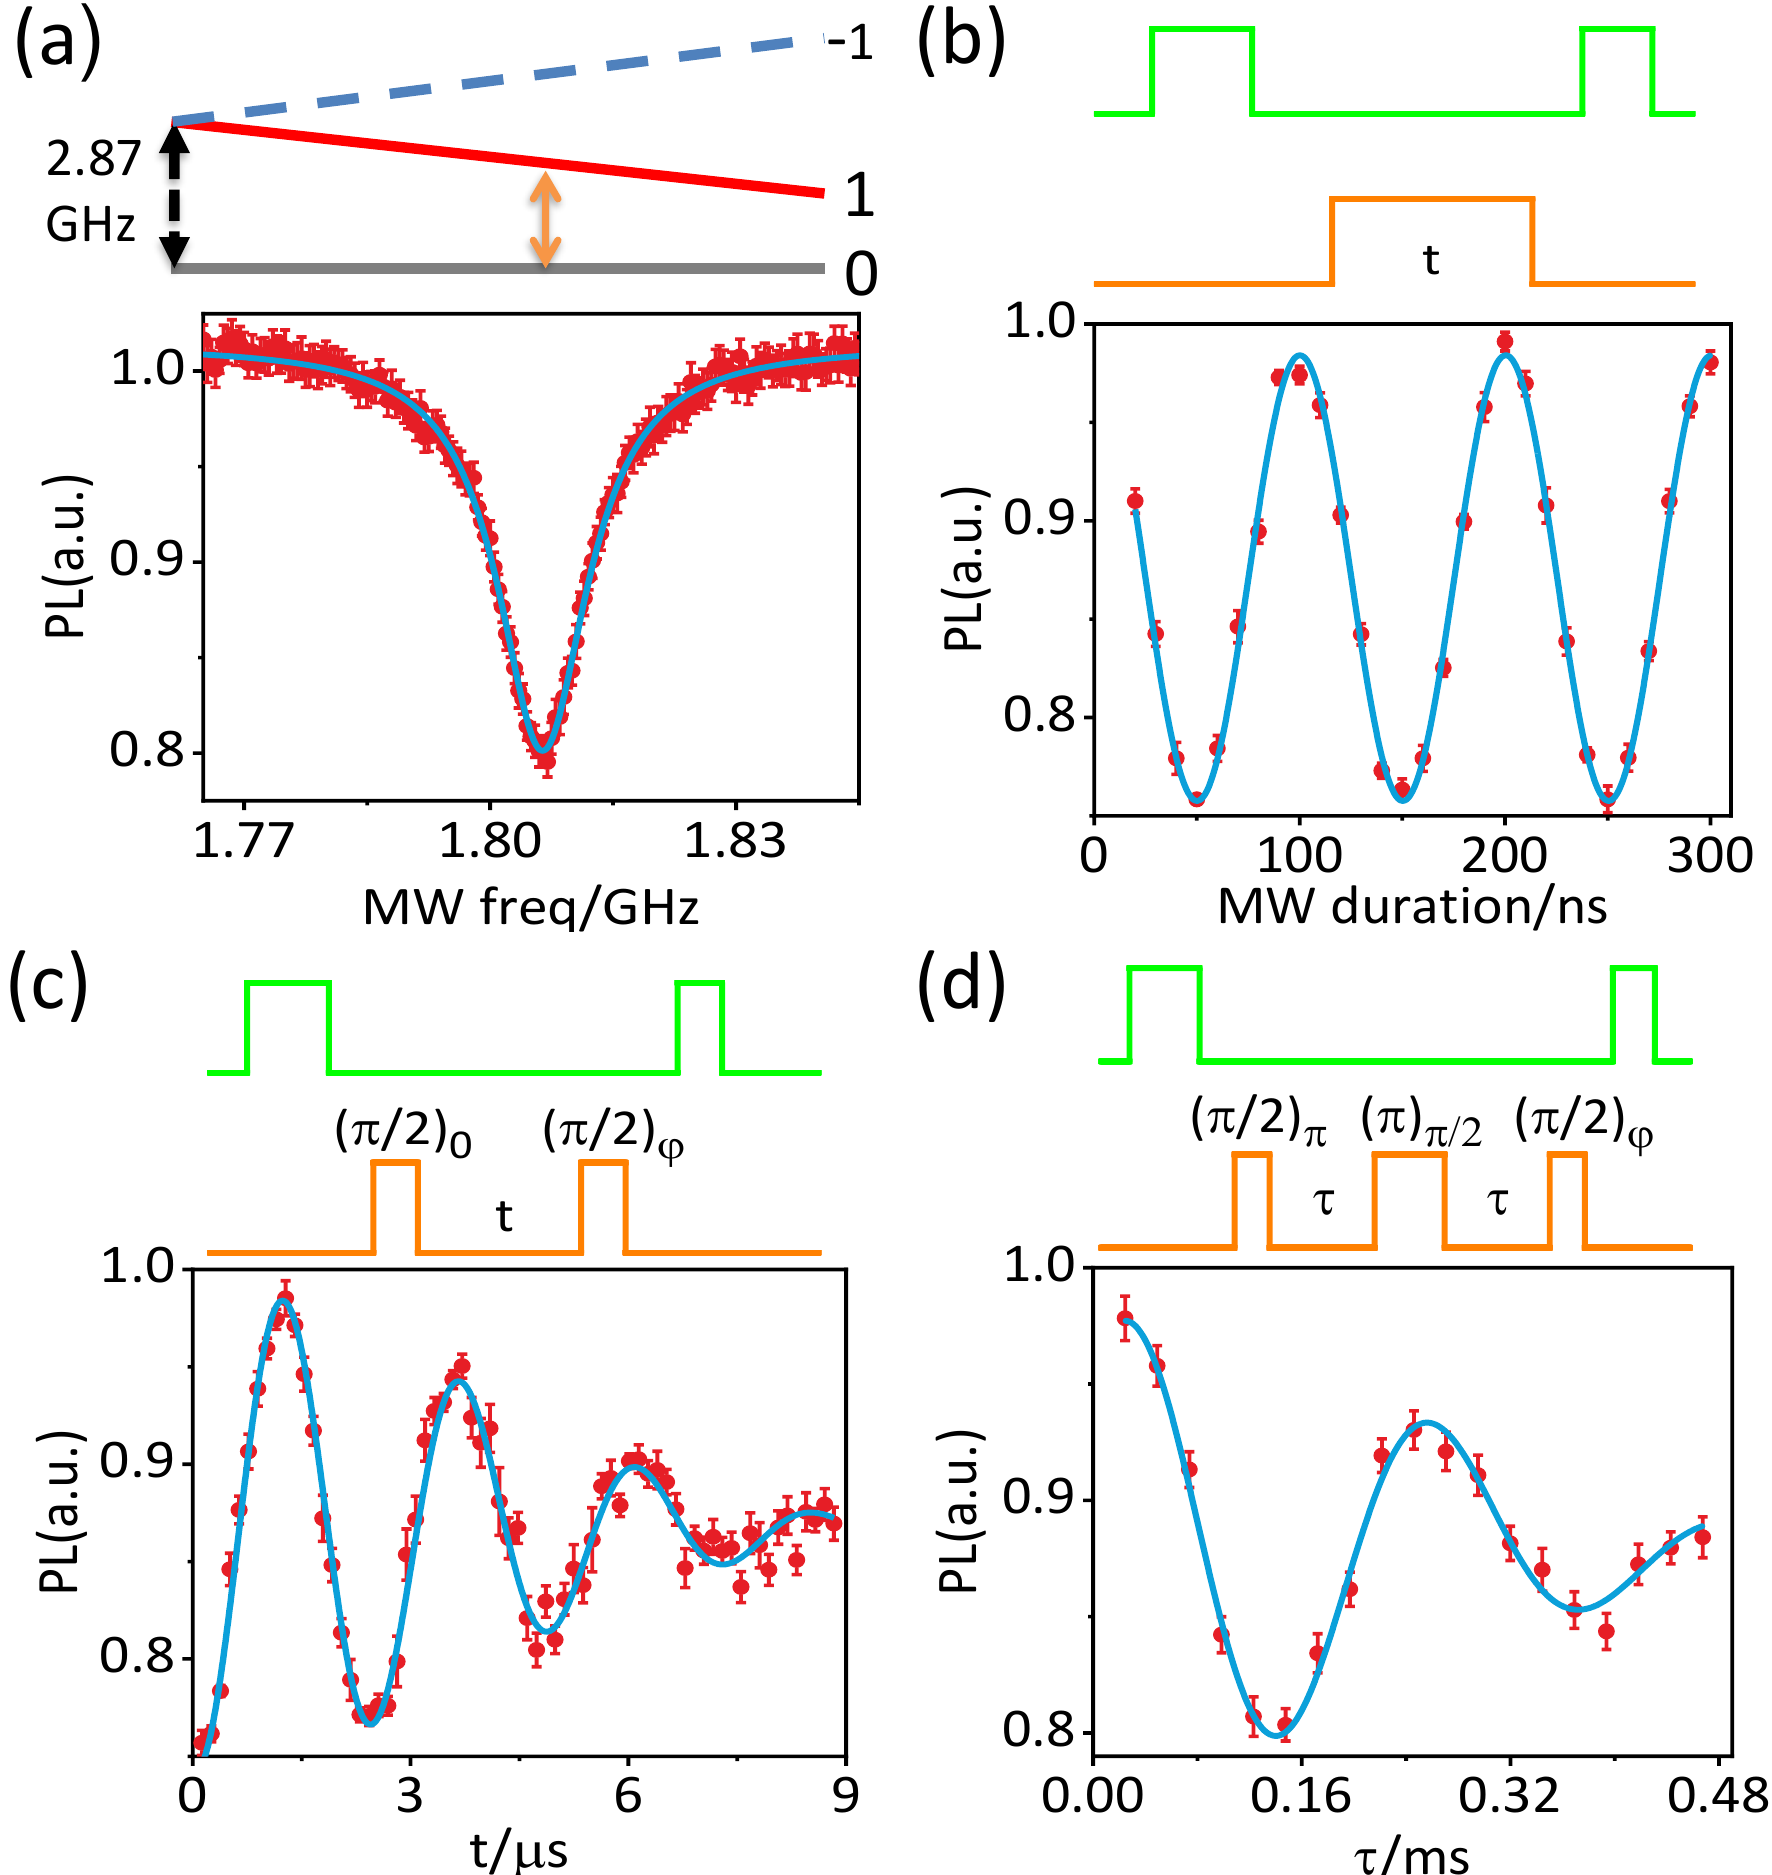}}
\caption{(a) Energy-level diagram of the NV center under external magnetic field ${B_0} $ (upper panel) and  the pulsed-ODMR spectrum
of $\left| 0 \right\rangle  \leftrightarrow \left| 1 \right\rangle $ with ${B_0} \approx 38$ mT (lower panel). The transition frequencies for $\left| 0 \right\rangle  \leftrightarrow \left| 1 \right\rangle $  is $1.806$ GHz. (b) Results of the nutation experiment for the electron spin and Rabi frequency is $\Omega  = 10$ MHz.  (c) FID of the electron spin with an dephasing time $T_2^* = 5.2(1)$ $\mu s$. (d) Spin echo pulse sequence used for coherence time measurement with ${T_2} = 0.66(2)$ ms.}
\label{Sfig1}
\end{figure}

\section{NV center in diamond}

The negatively charged NV center in diamond, where a substitutional nitrogen atom is next to a
vacancy, forms a spin triplet system in its ground state as shown in Fig. \ref{Sfig1}(a). Conveniently,
the NV spin can be initialized using optical pumping under green laser excitation and
optically read out by its spin-dependent fluorescence with a home-built confocal
microscopy at room-temperature. The NV's spin sub-levels of ground state are $\left| 0 \right\rangle $ and $\left| { \pm 1} \right\rangle $. The zero-field splitting between $\left| 0 \right\rangle $ and degenerate $\left| { \pm 1} \right\rangle $ sub-levels is ${\text{D = 2}}{\text{.87}}$ GHz. In
the experiment, we apply a strength of the external magnetic field near the excited
state level anti-crossing \cite{dong2018non}, i.e., ${{B}_0} \approx 38$ mT along the NV symmetry axis to split the energy
levels and polarize intrinsic $^{14}{N}$ nuclear spin to enhance the signal contrast up to ${C = 0.25}$.

We use a room-temperature home-built confocal microscopy, with a dry objective lens (N.A. $= 0.95$ Olympus), to image, initialize and read out NV center in a single-crystal synthetic diamond sample. The NV centers studied in this work are formed during chemical vapour deposition growth. The abundance of $^{13}C$ was at the nature level of $1$\%. Single NV centers are identified by observing anti-bunching in photon correlation measurements and the measurement of the spin splitting at zero magnetic field. The NV center is mounted on a three-axis closed-loop piezoelectric stage for sub-micrometre-resolution scanning. Fluorescence photons (wavelength ranging from $647$ to $800$ nm) are collected into a fiber and detected using single-photon counting module, with a counting rate of
$50$ kHz and a signal-to-noise ratio of $50:1$. A copper wire of $10$ $\mu m$ diameter above on the bulk diamond is used for the delivery of MW and arbitrary waveform to the NV center. The driving MW is generated by an AWG (Keysight M8190a) and amplified by a microwave amplifier (Mini-circuits ZHL-5W-2G-S+). The optical and MW pulse sequences are synchronized by a multichannel pulse generator (Spincore, PBESR-PRO-500).

Electron spin states $\left| 0 \right\rangle$ and $\left| 1 \right\rangle $ of NV center are encoded as the sensor qubit. Under resonance condition, the Rabi frequency
is set to be $\Omega  = 10$ MHz in experiment, as shown in Fig. \ref{Sfig1}(b). The undesired couplings between the NV center and the surrounding
$^{13}{C}$ nuclear spins lead to the effective dephasing effect. The resulting
free induction decay (FID) of the NV center is depicted in Fig. \ref{Sfig1}(c), where a dephasing
time $T_2^* = 5.2(1)$ $\mu s$ is obtained. The coherence
times ${T_2} = 0.66(2)$ ms is observed, as shown in Fig. \ref{Sfig1}(d).

\section{Quantum sensing of Arbitrary Waveforms}

The time-domain quantum difference (TDQD) protocol follows a general sequence of sensor initialization, interaction with the waveform, sensor readout, and  signal estimation. This sequence can be
summarized in the following basic protocol:
\begin{enumerate}[Step 1:]
  \item The quantum sensor is initialized into a known ground state, for example, $\left| 0 \right\rangle $.
  \item The quantum sensor is transformed into the desired initial sensing state $\left| \psi  \right\rangle {\text{ = }}\frac{{\left| 0 \right\rangle  + \left| 1 \right\rangle }}{{\sqrt 2 }}$ with a $\frac{\pi }{2}$ pulse.
  \item The superposition state evolves under the magnetic field $b(t)$ that we aim to measure at a time $t_i$. The superposition state picks up the relative phase: $$\phi(t_i)  = \int_0^{t_i} {{\gamma _e}b(t)dt}  - \int_{t_i}^T {{\gamma _e}b(t)dt}  - \int_0^{{t_i} + {t_s}} {{\gamma _e}b(t)dt}  + \int_{{t_i} + {t_s}}^T {{\gamma _e}b(t)dt}  =  - 2\int_{t_i}^{{t_i} + {t_s}} {{\gamma _e}b(t)dt} .$$ For ${t_s}/T \ll 1$, we have $\phi ({t_i}) \approx  - 2{\gamma _2}b({t_i}){t_s}$.
  \item Using a second $\frac{\pi }{2}$ pulse, the relative phase is mapped into x-y plane of Bloch sphere.
  \item The final state of the quantum sensor is read out by employing the initial phase of Rabi oscillation.
\end{enumerate}
Steps 1--5 represent a single measurement cycle. To reduce the fluctuation of detection signal, the measurement cycle needs to be repeated many times ($2 \times {10^6}$) in experiment. And we can control the repetition times ($k$) of Step 3 to linearly increase the accumulation relative phase (${\phi _{{n_2}}} = k\phi({t_i}) $). The number of resources used in TDQD protocol is ${n_2} = 2k$ for each sampling. The whole pulse sequences are shown in Fig. \ref{Sfig2}(a) based on NV center sensor in diamond. Fig. \ref{Sfig2}(b) shows the basic dynamic evolution of quantum sensor qubit with a Bloch sphere. The sensor outputs $s(t)$ for a serial of $k$ values of the two-$\pi$-pulse unit in the estimation of a sinusoidal waveform with period of $T = 2.4$ $\mu s$. The integration time and $\pi$-pulse duration are $t_{s}=300$ ns and $t_{\pi} = 50$ ns, respectively.

\begin{figure}[tbp]
\centering
\textsf{\includegraphics[width=15cm]{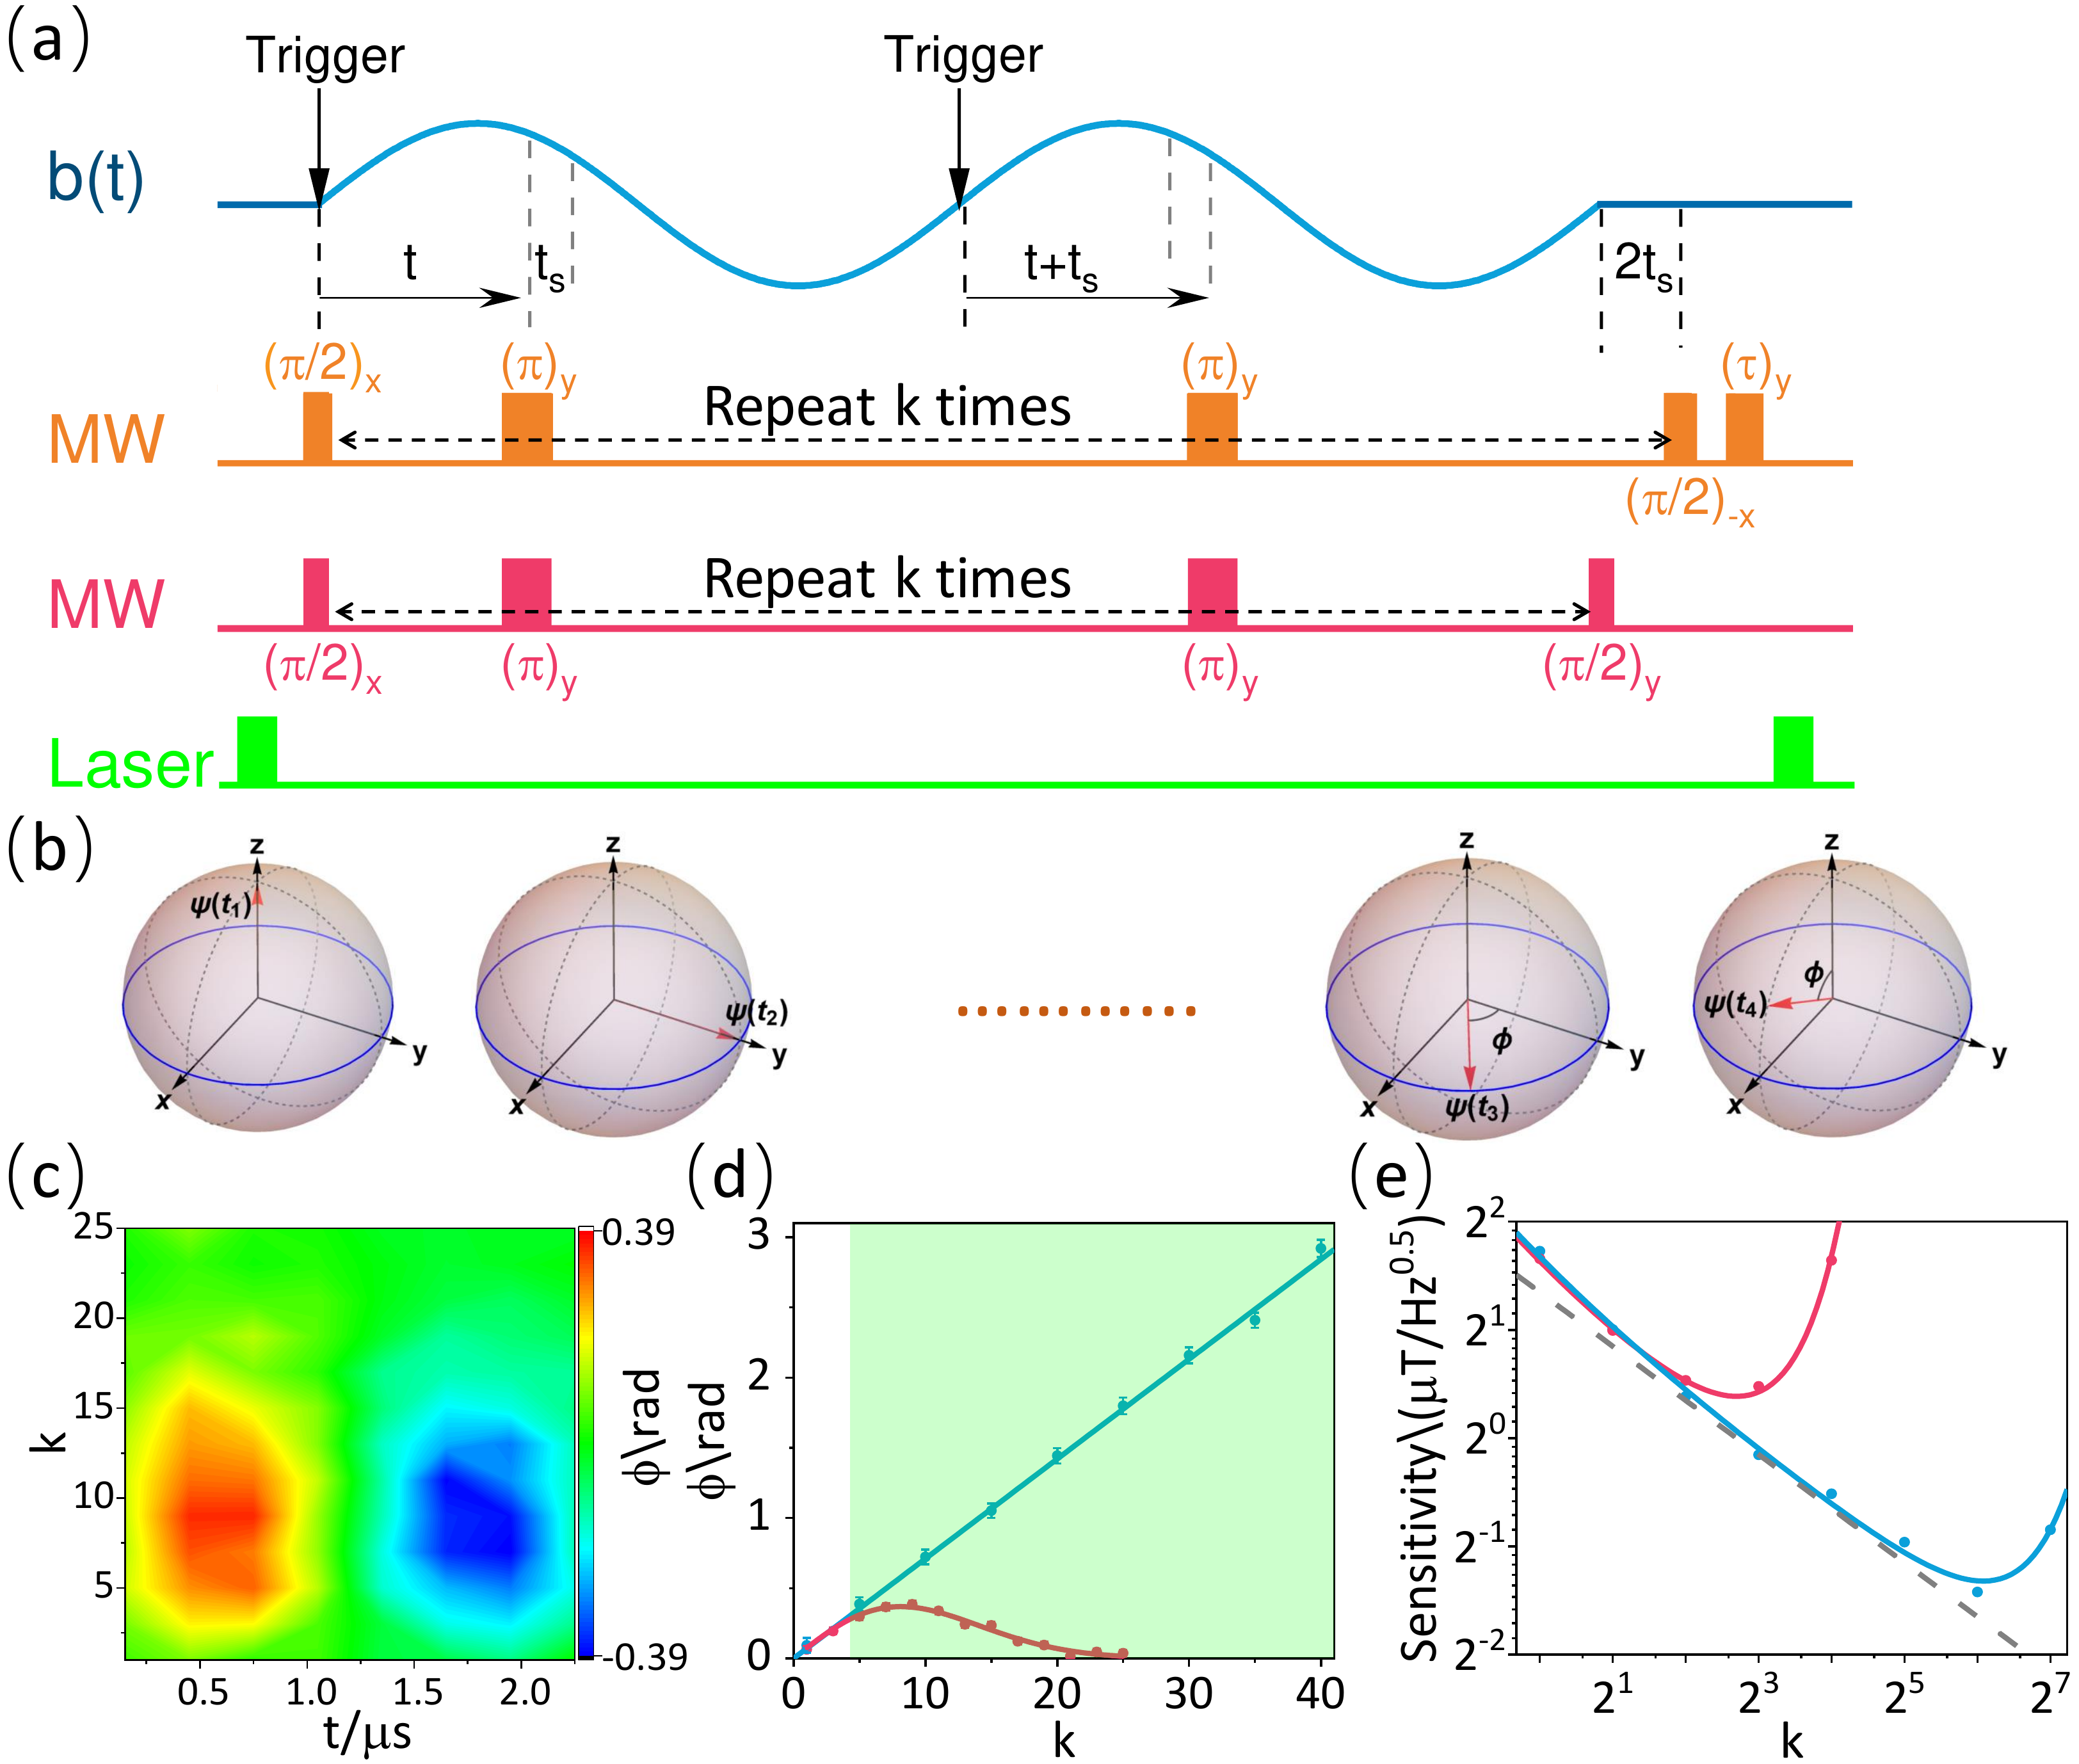}}
\caption{(a) Pulse sequence for waveform sampling. Based on PDD, we propose the robust TDQD detection method (orange pulse train). By scanning the moment of applying $\pi$ gates, the arbitrary waveform can be reconstructed. As a comparison, the original TDQD protocol is plotted with pink. (b) Dynamically process of TDQD protocol with Bloch sphere. (c) Increased sensitivity by integrating $2k$ waveform passages with the differential spin-echo detection. (d-e) Comparison of two arbitrary waveform estimation protocols. Red (blue) lines and dots show the theoretical and experimental results with (PDD-enhanced) TDQD protocol.}
\label{Sfig2}
\end{figure}

In the original protocol of reconstruction-free quantum sensing of arbitrary waveforms \cite{PhysRevApplied.12.054028}, the only idea of unwanted dynamic evolution coherent cancellation is exploited with two-$\pi $-pulse block as shown in Fig. \ref{Sfig2}(a) with pink pulse train. The signal of the waveform sampling at ${t_i}$ can be expressed as:
\begin{equation}
s\sim\exp \left[ { - {{\left( {\frac{{2k{t_s}}}{{T_2^*}}} \right)}^2}} \right]\exp \left[ { - {{\left( {\frac{{2kT}}{{{T_2}}}} \right)}^2}} \right]\sin 2k{\phi _i} \text{.}
\end{equation}
For small value $k$, $s\sim\exp \left[ { - {{\left( {\frac{{2k{t_s}}}{{T_2^*}}} \right)}^2}} \right]\exp \left[ { - {{\left( {\frac{{2kT}}{{{T_2}}}} \right)}^2}} \right]2k{\phi _i}$ \cite{PhysRevApplied.12.054028}. Due to dephasing effect and simple accumulation phase readout method, the sensitivity (4 $\mu T/\surd Hz$) and dynamic range ($\left[ {0,0.05} \right]$ rad) of reconstruction waveform is limited seriously based on the original TDQD protocol \cite{PhysRevApplied.12.054028} in practice. We repeat the TDQD protocol, and the results are shown in Fig. \ref{Sfig2}(c). Clearly, with the increasing value of $k$, the TDQD method would be invalid in experiment.

In this work, we directly improve the differential-waveform sampling with periodic dynamical decoupling (PDD) method \cite{PhysRevLett.106.240501}, which is a powerful technique for protecting qubits in quantum computing and quantum memory from the environment. The decay time constant of signal can be directly obtained and the signal for our protocol is
\begin{equation}
s \sim \exp \left[ { - {{\left( {\frac{{2k\left( {T + {t_{s}}} \right)}}{{{T_2}}}} \right)}^2}} \right]\cos 2k{\phi _i}\text{.}
\end{equation}

\begin{figure}[bp]
\centering
\textsf{\includegraphics[width=8.5cm]{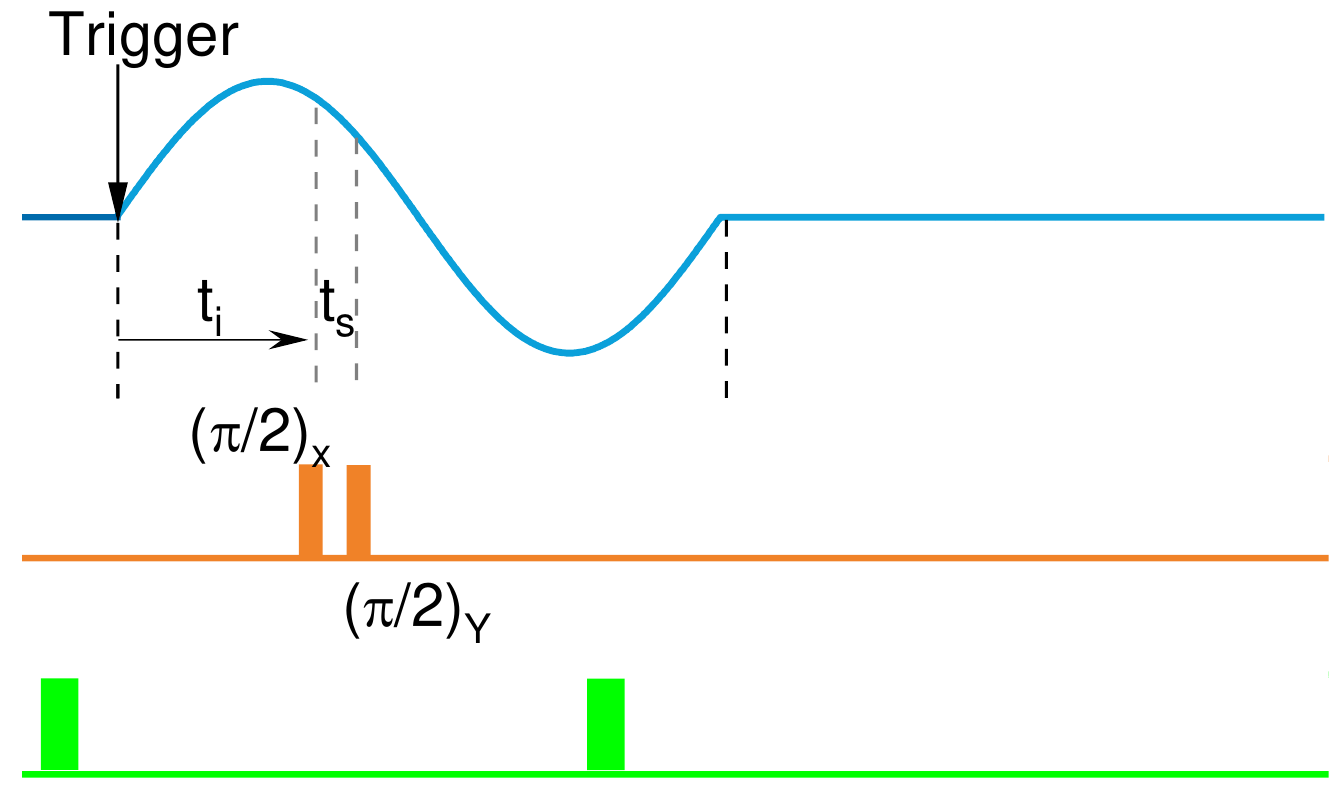}}
\caption{Pulse sequence for the SQL measurement of waveform sampling. This sensor sequence was repeated for given numbers as shown in Fig. 3(a) of main text.}
\label{Sfig3}
\end{figure}

So the PDD-enhanced TDQD protocol can coherently amplify accumulation phase, cancel unwanted coherent dynamical evolution and suppress quantum decoherence simultaneously. Beside those advantages, the PDD-enhanced TDQD is also immune to imperfect pulse error operation. The green shadow region in Fig. \ref{Sfig2}(d) denotes the dynamic range improvement of the PDD-enhanced TDQD protocol. To quantify the sensitivity in the presence of decoherence and sensor readout overhead, we calculate a minimum detectable field $B_{min}$ \cite{PhysRevApplied.12.054028}, defined as the input waveform that gives a unity signal-to-noise ratio for a given integration time, as shown in Fig. \ref{Sfig2}(e). To suppress the pure dephasing effect of $^{13}C$ further, the period of unknown arbitrary waveform should satisfy ${{\gamma _{^{13}C}}}{B_0}T \approx 2m\pi $ for NV center in diamond, where $m$ is a positive integer number. Assisting with $^{12}C$-enriched growth technology \cite{ISI000482888200001}, this constraint condition can be totally dropped.

\begin{figure}[tbp]
\centering
\textsf{\includegraphics[width=12cm]{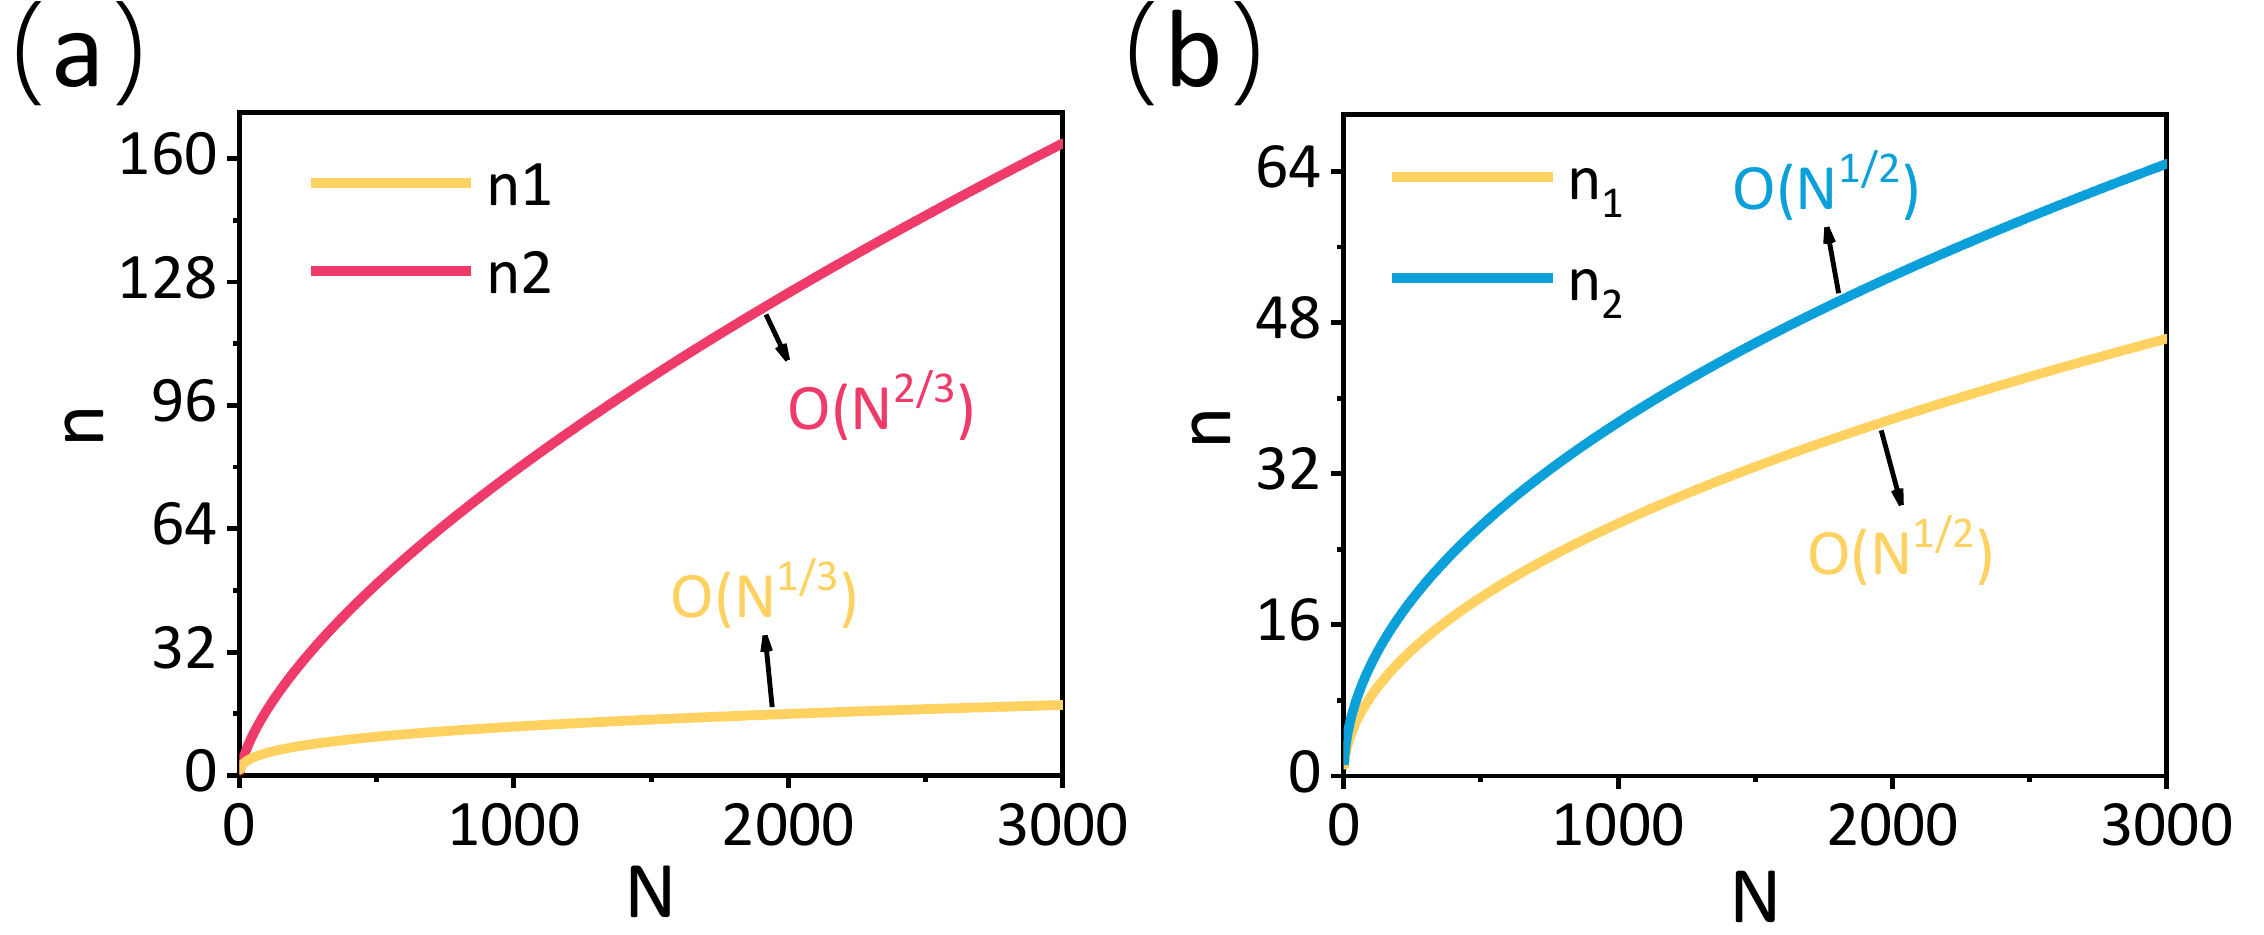}}
\caption{(a)(b) The best allocation of quantum resource for waveform estimation with SQL or HQL scheme, respectively.}
\label{Sfig4}
\end{figure}

For the SQL in arbitrary waveform estimation, the small-interval ramsey detection is employed to avoid numerical processing as shown in Fig. \ref{Sfig3}. To perfectly demonstrate the advantage of HQL in arbitrary waveform estimation with our current technology, we
chose a $1$th-order differentiable waveform in experiment. And the period of waveform approximately satisfies ${\gamma _{^{13}c}}{B_0}T \approx 8\pi $, where $T = 9.6$ $\mu s$. The maximal number of samples in one period is ${n_1} = \frac{T}{{{t_s} + 2{t_\pi }}}\sim64$, where ${{t_{s }}=150}$ ns. So, the multi-round number is ${n_2} = \frac{T}{{T_2}} \approx {n_1}$. By fitting experimental results in Fig.3(a) in the main text, the scaling laws show ${\delta _{stat}} = {0.0555/}\sqrt {{{n}_2}}$ (${\delta _{stat}} = {0}{.0555/}{{n}_2}$) for SQL (HQL) and  ${\delta _{\det }}{= 0}{.04/}{{n}_1}$. Since the overall error is ${\delta ^2}=\delta _{det}^2 + \delta _{stat}^2$, the best allocation of quantum resource for the waveform estimation can be calculated with numerical method and results are shown in Fig. \ref{Sfig4}(a) and (b). In experiment, we exploit numerical approximate rounding method \cite{NoceWrig06} to get the best quantum resource allocation approximately as shown in Tables \uppercase\expandafter{\romannumeral1}--\uppercase\expandafter{\romannumeral2} and Fig. 3(b) in the main text.

\begin{table}[h]
\centering
\caption{Optimal resource allocation of SQL scheme.}
\tabcolsep0.06in
\begin{tabular}{cccccccccc}
  \hline
  \hline
  NO. & 1 & 2 & 3 & 4 & 5 & 6  & 7 & 8 & 9 \\
  \hline
  $N$ & 4 & 32 & 60 & 168 & 480 & 840 & 1066 &1984 & 2380\\
  \hline
  ${{n}_1}$ & 2 & 4 & 5 & 7 & 10 & 12 & 13 & 16 & 17  \\
  \hline
  ${{n}_2}$ & 2 & 8 & 12 & 24 & 48 & 70 & 82 & 124 & 140  \\
  \hline
  \hline
\end{tabular}
\end{table}

\begin{table}[h]
\centering
\caption{Optimal resource allocation of HQL scheme.}
\tabcolsep0.06in
\begin{tabular}{ccccccccccccc}
  \hline
  \hline
  NO. & 1 & 2 & 3 & 4 & 5 & 6  & 7 & 8 & 9 & 10 & 11 & 12\\
  \hline
  $N$ & 12 & 140 & 234 & 408 & 560 & 736 & 1026 &1260& 1518 & 1924 & 2240 & 2580 \\
  \hline
  ${{n}_1}$ & 3 & 10 & 13 & 17 & 20 & 23 & 27 & 30 & 33 & 37 & 40 & 43 \\
  \hline
  ${{n}_2}$ & 4 & 14 & 18 & 24 & 28 & 32 & 38 & 42 & 46 & 52 & 56 & 60 \\
  \hline
  \hline
\end{tabular}
\end{table}

\end{document}
